# Supplementary material for: CrossViT: Cross-Attention Multi-Scale Vision Transformer for Image Classification
Source: arXiv:2103.14899 source file (2021-08-22)
Supplement: Supplementary file 1 [file c1.tex]

% \begin{table}[t]
%     \centering
%     \begin{adjustbox}{max width=\linewidth}
%     \begin{tabular}{l|c|c}
%         \toprule
%         % Tiny    & DeiT     & CrossViT \\
%         % \midrule
%         % Linear  &  72.2/1.3/5.7  & 73.4/1.6/6.9  \\
%         % Three Convolutions  & 75.3/1.3/5.8  &  74.7/1.6/7.1 \\
%         % Three Convolutions  & 74.4/1.3/5.8  &  74.7/1.6/7.1 \\
        
%         % \midrule
%         % \midrule
%         9    & DeiT     & CrossViT \\
%         \midrule
%         Linear  &  72.9/1.4/6.4  & 73.9/1.8/8.6  \\
%         3 Convs.  & 75.6/1.5/6.6  &  77.1/2.0/8.8 \\
%         % \midrule
%         % \midrule
%         % Small    & DeiT     & CrossViT \\
%         % \midrule
%         % Linear  &  79.8/4.6/22.1  & 81.0/5.6/26.7  \\
%         % Three Convolutions  & 81.6/4.8/22.6  &  82.1/5.6/26.7 \\
%         \midrule
%         \midrule
%         %  DeiT     & CrossViT \\
%         \midrule
%         15    & Linear  &  80.8/4.9/22.9  & 81.5/5.8/27.4  \\
%         3 Convs.  & 81.7/5.1/23.5  & 82.3/6.1/28.2 \\
%         \midrule
%         \midrule
%         18    & DeiT     & CrossViT \\
%         \midrule
%         Linear  &  81.4/7.8/37.1  & 82.5/9.0/43.3  \\
%         3 Convs.  & 81.2/8.1/37.9  & 82.8/9.5/44.3 \\
%         \bottomrule
%     \end{tabular}
%     \end{adjustbox}
%     % \vspace{-2mm}
%     \caption{\textbf{Comparisons with DeiT baseline on ImageNet1K.}}
%     \label{table:xx}
% \end{table}

\begin{table}[t]
    \centering
    \begin{adjustbox}{max width=\linewidth}
    \begin{tabular}{l|c|c}
        \toprule
        % Tiny    & DeiT     & CrossViT \\
        % \midrule
        % Linear  &  72.2/1.3/5.7  & 73.4/1.6/6.9  \\
        % Three Convolutions  & 75.3/1.3/5.8  &  74.7/1.6/7.1 \\
        % Three Convolutions  & 74.4/1.3/5.8  &  74.7/1.6/7.1 \\
        
        % \midrule
        % \midrule
        9    & DeiT     & CrossViT \\
        \midrule
        Linear  &  72.9/1.4/6.4  & 73.9/1.8/8.6  \\
        3 Convs.  & 75.6/1.5/6.6  &  77.1/2.0/8.8 \\
        % \midrule
        % \midrule
        % Small    & DeiT     & CrossViT \\
        % \midrule
        % Linear  &  79.8/4.6/22.1  & 81.0/5.6/26.7  \\
        % Three Convolutions  & 81.6/4.8/22.6  &  82.1/5.6/26.7 \\
        \midrule
        \midrule
        15    & DeiT     & CrossViT \\
        \midrule
        Linear  &  80.8/4.9/22.9  & 81.5/5.8/27.4  \\
        3 Convs.  & 81.7/5.1/23.5  & 82.3/6.1/28.2 \\
        \midrule
        \midrule
        18    & DeiT     & CrossViT \\
        \midrule
        Linear  &  81.4/7.8/37.1  & 82.5/9.0/43.3  \\
        3 Convs.  & 81.2/8.1/37.9  & 82.8/9.5/44.3 \\
        \bottomrule
    \end{tabular}
    \end{adjustbox}
    % \vspace{-2mm}
    \caption{\textbf{Comparisons with DeiT baseline on ImageNet1K.}}
    \label{table:xx}
\end{table}
