# Supplementary material for: CrossViT: Cross-Attention Multi-Scale Vision Transformer for Image Classification
Source: arXiv:2103.14899 source file (2021-08-22)
Supplement: Supplementary file 2 [file c2.tex]

\begin{table}[t]
    \centering
    \begin{adjustbox}{max width=\linewidth}
    \begin{tabular}{l|cc|cc|cc}
        \toprule
        Model    & \multicolumn{2}{c}{Top-1 Acc (\%)} & \multicolumn{2}{c}{FLOPs (G)} & \multicolumn{2}{c}{Params (M)} \\
                 & Baseline & Method & Baseline & Method & Baseline & Method \\ 
        \midrule
        PVT-S & 79.9 & 79.8 (-0.1) & 4.6 & 3.8 & 22.1 & 24.5 \\
        \midrule
        CentroidViT & 79.9 & 80.9 (+1.0) & 4.7 & 4.7 & 22.1 & 22.3 \\
        \midrule
        TNT-S    & 79.8 & 81.3 (+1.5) & 4.6  & 5.2 & 22.1 & 23.8  \\
        % TNS-B    & 81.8 & 82.8 (+1.0) & 86.4 & 65.6 & 17.6 & 14.1 \\
        \midrule
        T2T-ViT-14 & 78.9 & 80.7 (+1.8) & 4.3 & 6.1 & 21.1 & 21.4 \\
        \midrule
        \ours-S  &  79.8 & 81.0 (+1.2) & 4.6 & 5.6 & 22.1 & 26.7  \\
        \ours-S$\dagger$  &  79.8 & 82.1 (+2.3) & 4.8 & 5.6 & 22.1 & 27.1  \\
        \bottomrule
    \end{tabular}
    \end{adjustbox}
    % \vspace{-2mm}
    \caption{\textbf{Comparisons with its own referenced baseline on ImageNet1K.} We list the performance of their method with minimal changes to the baseline. This could clearly to check the improvement over the proposed methods.}
    \label{table:xx}
\end{table}
